# Supplementary material for: Charge density wave induced nodal lines in LaTe$_3$
Source: arXiv:2212.01181 source file (2022-12-02)
Supplement: Supplementary file 1 [file Supplementary_optimized.pdf]

# Supplementary information for "Charge density wave induced nodal lines in $LaTe_3$"

Shuvam Sarkar[1], Joydipto Bhattacharya[2,3], Pampa Sadhukhan[1], Davide Curcio[4], Rajeev Dutt[2,3], Vipin Kumar Singh[1], Marco Bianchi[4], Arnab Pariari[5], Shubhankar Roy[6], Prabhat Mandal[5], Tanmoy Das[7], Philip Hofmann[4], Aparna Chakrabarti[2,3], Sudipta Roy Barman[1]

[1]*UGC-DAE Consortium for Scientific Research, Khandwa Road, Indore 452001, Madhya Pradesh, India*

[2]*Theory and Simulations Laboratory, Raja Ramanna Centre for Advanced Technology, Indore 452013, Madhya Pradesh, India*

[3]*Homi Bhabha National Institute, Training School Complex, Anushakti Nagar, Mumbai 400094, Maharashtra, India*

[4]*Department of Physics and Astronomy, Interdisciplinary Nanoscience Center (iNANO), Aarhus University, 8000 Aarhus C, Denmark*

[5]*Saha Institute of Nuclear Physics, HBNI, 1/AF Bidhannagar, Kolkata 700 064, India*

[6]*Vidyasagar Metropolitan College, 39, Sankar Ghosh Lane, Kolkata 700006, India and*

[7]*Department of Physics, Indian Institute of Science, Bangalore, 560012, India*

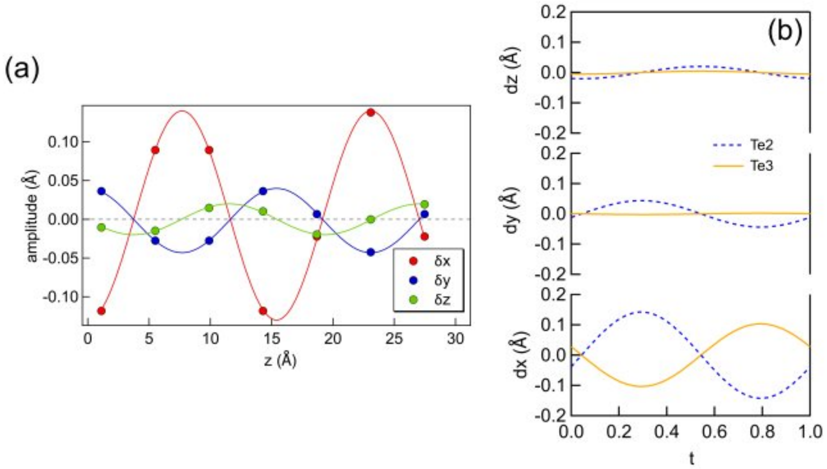


FIG. S1. **CDW modulations in the Te net.** (a) Positions of the Te2 atoms in the 7-fold modulated structure of $LaTe_3$, where $\delta x$, $\delta y$ and $\delta z$ are the displacements from the non-CDW positions along $x$, $y$ and $z$ directions, respectively. (b) The displacements of Te atoms along the three directions from XRD [2]. Note that $\delta x = 0.135$ Å from the 7-fold structure is quite similar to that obtained from XRD (0.142 Å). Even the smaller CDW amplitudes ($\delta y = 0.042$ and $\delta z = 0.02$ Å) are close to the experimental values (0.047 and 0.02 Å, respectively).

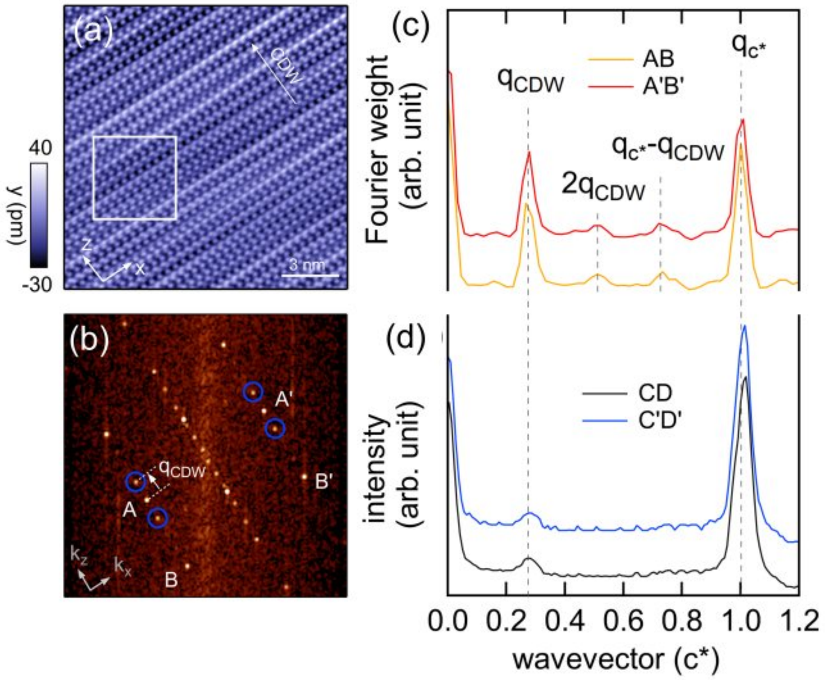


FIG. S2. $q_{\rm CDW}$ **from STM and LEED.** (a) A large area ($14.7\times14.7$ nm$^2$) scanning tunneling microscopy (STM) topography in the CDW state of $LaTe_3$ measured in the constant current mode with bias voltage of 0.2 V and a tunneling current of 0.4 nA. The zoomed image of the enclosed area inside the white box is shown in Fig. 1b. (b) Fourier transform of the STM image, where the CDW related satellite spots are encircled. The intensity line profiles from (c) the FFT of the STM image shown in panel **b** and (d) the low energy diffraction (LEED) pattern shown in Fig. 1c of the main text.

## Supplementary Note 1:
## Determination of $q_{\rm CDW}$ from scanning tunneling microscopy and low energy electron diffraction

A scanning tunneling microscopy (STM) topography image in Supplementary Fig. S2a reveals the topmost Te layer, a zoomed image (white square) is shown in Fig. 1b of the main text. In Supplementary Fig. S2b, the Fourier transform of the STM image in panel **a** shows the CDW related satellite spots (blue circles) along $c^*$. The intensity line profiles along AB and A′B′ in Supplementary Fig. S2c gives $q_{\rm CDW} = 0.28\pm0.02c^*$ that is related to the first satellite peak.

Intensity profiles through CD and C′D′ (Fig. S2d) of the low energy electron diffraction (LEED) pattern in Fig. 1c provide the estimate of $q_{\text{CDW}}$ to be $0.275\pm0.001c^*$, in good agreement with ARPES (Supplementary Figs. S4a,b) and STM (Supplementary Fig. S2c). Furthermore, the closeness of $q_{\text{CDW}}$ between the surface sensitive measurements (ARPES, STM and LEED) and bulk-sensitive XRD [2] is consistent with the 2D nature of $LaTe_3$.

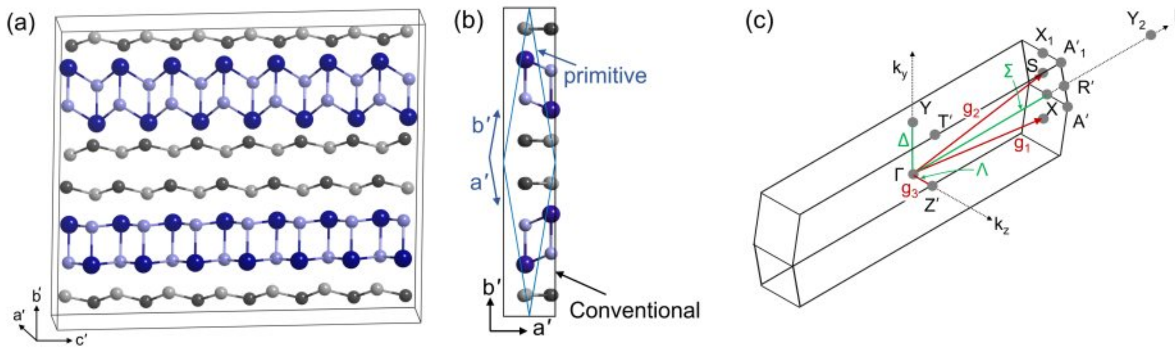


FIG. S3. **The unit cell and Brillouin zone of $LaTe_3$ in the CDW state.** (a) The *conventional* i.e., non-primitive unit cell of the 7-fold modulated structure with 112 atoms and $a'_c$= 4.378, $b'_c$= 26.149, $c'_c$= 30.778 Å, $\alpha'_c$= $\beta'_c$= $\gamma'_c$= 90°. A comparison with the lattice parameters of the *conventional* i.e., non-primitive unit cell of the non-CDW state with $a_c$= 4.378, $b_c$= 26.149, and $c_c$= 4.397 Å shows that $c'_c$ is 7 times larger than $c_c$ due to the 7-fold modulation. Also it is the convention in $RTe_3$ to take $b_c$ as the vertical long axis, with Te bilayer in the $a_c$-$c_c$. (b) A comparison of the conventional and the primitive unit cell in the CDW state viewed along the $c'$ axis. (c) Brillouin zone (BZ) of the 7-fold structure of the CDW-state (ordering of the conventional lattice: $a'_c < b'_c$ [9]) showing the primitive reciprocal lattice vectors $g_1$, $g_2$ (both in $k_x$-$k_y$ plane) and $g_3$ (along $k_z$). The co-ordinates of the high symmetry points/lines in terms of the primitive reciprocal lattice vectors are as follows: Γ (0,0,0), $X$ ($\zeta$,$\zeta$,0) where $\zeta$= 0.257 = $0.25(1+a'^2/b'^2)$, $Z'$ (0,0,0.5), $Y$ (-0.5,0.5,0), $A'$ ($\zeta$,$\zeta$,0.5), $A'_1$ (-$\zeta$,1-$\zeta$,0.5), $T'$ (-0.5,0.5,0.5), $S$ (0,0.5,0), $R'$ (0,0.5,0.5), $X_1$ (-$\zeta$,1-$\zeta$,0) and lines Δ ($-u$,$u$,0), Λ (0,0,$u$), Σ ($u$,$u$,0), $P$ ($u$,$v$,0), and $M$ ($u$,$u$,$v$). $Y_2$ i.e., the $Y$ point in the next BZ along Σ is given by (0.5,0.5,0).

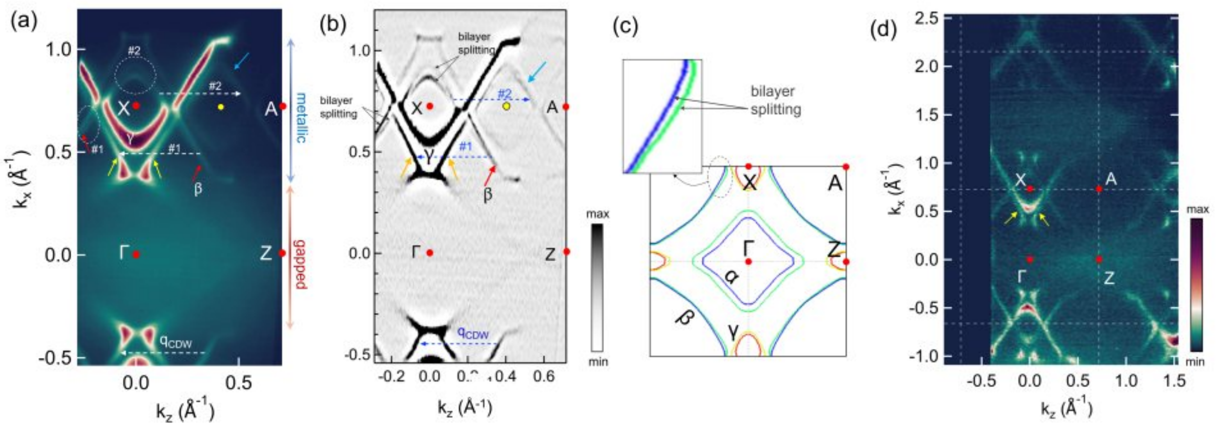

FIG. S4. **Fermi surface from ARPES at 100 K.** (a) The Fermi surface (FS) of $LaTe_3$ in the CDW state using photon energy (h$\nu$) of 24.4 eV. The gapped and the metallic parts of the FS are marked by red and blue double arrows on the right axis, respectively. The white dashed arrows of length by $q_{\rm CDW}$ connect some of the shadow branches with the main branches of the FS. The high symmetry points of the BZ (both CDW and non-CDW, see Fig. 1d of the main manuscript) are indicated. (b) A curvature plot of the FS shown in panel **a**, where the weak shadow FS pockets are visible. The blue dashed arrows indicate the $q_{\rm CDW}$. (c) The calculated FS in the non-CDW state. The inset shows the bilayer splitting of the $\beta$ sheet. (d) A large area FS plot measured using h$\nu$= 80 eV.

## Supplementary Note 2: Fermi surface of $LaTe_3$ in CDW state measured by ARPES

*Shadow branches and determination of $q_{\rm CDW}$:* The Fermi surface (FS) in Supplementary Figs. S4a,b reveals the presence of weak FS branches highlighted by yellow arrows in the metallic part of the FS, besides the main branches. These are also observed in a larger area FS taken with 80 eV photon energy, see Supplementary Fig. S4d. The main branches are related to the main bands that are present in the non-CDW state, but the weak branches are absent in the calculated FS of the non-CDW state (Supplementary Fig. S4c, the different Fermi sheets are shown) indicating that these are related to the CDW state. These

are nearly parallel to the sides of the $\gamma$ pocket and connect with the ungapped corner of the $\alpha$ sheet. The ungapped portions of the outer $\beta$ sheet (red arrows in Supplementary Figs. S4a,b) are also observed. If the $\beta$ sheet is compared with the weak FS branch, it is clear that the latter is a replica of the former, but shifted by $q_{\text{CDW}}$, as shown by a horizontal dashed white/blue arrow (#1). Moreover, a weak diamond shaped FS contour (one side denoted by blue arrow) is observed around the yellow dot, which is the replica of the $\gamma$ pocket around the $X$ point, again shifted by $q_{\text{CDW}}$(white/blue dashed arrow #2). These additional branches (more prominent in the curvature plot in Supplementary Fig. S4b) are related to the shadow bands that arise due to the CDW periodicity [1]. The identification of the shadow branches of the FS allows a quantitative determination of $q_{\text{CDW}}$ by taking cuts along $k_z$ for different $k_x$. In this way, $q_{\text{CDW}}$ is found to be $0.28\pm0.005c^*$.

*Bilayer splitting:* Splitting of the FS branches are observed in the $\beta$ sheet (white dashed oval #1) and in the $\gamma$ pocket around $X$ (white dashed oval #2) in Supplementary Fig. S4a, which are more prominent in the curvature plot (Supplementary Fig. S4b). The splitting varies with $k$, e.g., for the $\gamma$ pocket it is maximum ( 0.05 Å$^{-1}$) along $\Gamma X$ ($\Sigma$ with coordinates ($u$,$u$,0) in terms of reciprocal lattice vectors, see Supplementary Fig. S3c) and becomes smaller for larger $k_z$. For the $\beta$ sheet, it decreases for larger $k_z$. In contrast to the shadow branches, the calculated FS for the non-CDW state also shows such a splitting, as shown for the $\beta$ sheet by a black dashed oval in Supplementary Fig. S4c and its inset. The splitting is also observed in the $\gamma$ pocket, but is most prominent for the $\alpha$ sheet (green and blue curves). Since the splittings are visible in both the states, these are not related to the CDW, but play an interesting role in giving rise to two types of nodal lines in $LaTe_3$.

*Gapped part of the FS around $\Gamma Z$:* The FS in Supplementary Fig. S4a shows a $k_x$= $\pm$0.4 Å$^{-1}$ region around the $\Gamma Z$ direction with no feature (vertical red double arrow on the right) in contrast to the metallic part (vertical cyan double arrow). This is because the FS here is gapped due to the CDW, in agreement with the ARPES band dispersion discussed in subsection II F of the main text (Fig. 4, Supplementary Figs. S4a,b and S6). In contrast, the calculated FS of the non-CDW state in Supplementary Fig. S4c shows two diamond

shaped sheets ($\alpha$ and $\beta$) around $\Gamma$ and four smaller oval pockets ($\gamma$) around $Z$ and $X$. The central part of the $\alpha$ and $\beta$ sheets is not observed in the experimental FS as these are in the gapped region. However, the $\gamma$ pocket around the $X$ point is visible in the metallic region.

## Supplementary Note 3: Bader charge analysis

TABLE S1. Bader charge analysis for $LaTe_3$.

| **No.** | **Atom** | **Net charge (e)** | |
|---|---|---|---|
| | | **non-CDW** | **CDW** |
| 1 | La1 | 1.503 | 1.539 |
| 2 | Te1 | -0.996 | -1.029 |
| 3 | Te2 | -0.252 | -0.254 |
| 4 | Te3 | -0.255 | -0.256 |

The transfer of electrons from La to the Te2-Te3 net determines the band filling and this has been calculated using the Bader charge analysis [4, 5]. The results for the CDW and the non-CDW state are nearly similar, as shown in the Supplementary Table S1. We find that 0.5 electronic charge from a La atom is transferred to the two Te atoms in the net and thus the valency of both Te2 and Te3 is -0.25 (outer shell configurations of La and Te atoms are $5d^1 6s^2$ and $5s^2 5p^4$, respectively). One electron is transferred from La to Te1. Thus, the valency of La is +1.5, while that of Te1 is -1. The present DFT results thus do not support the assumption in an earlier tight binding calculation [6] that La has +3 valency. The two different valencies of Te is experimentally verified by the difference in the $E$ of the Te2-Te3 and Te1 related peaks in the Te $4d$ core-level spectrum (Supplementary Fig. S5). The former

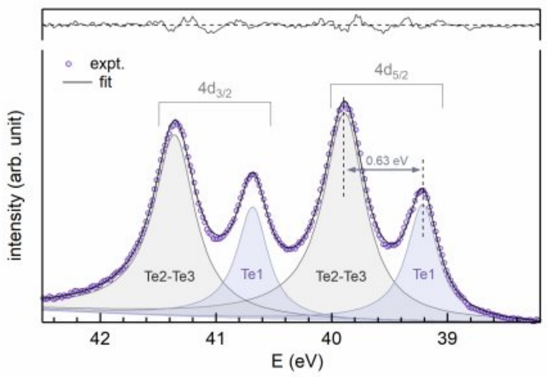


FIG. S5. **Te 4*d* core level spectrum.** Te $4d$ core level spectrum measured using h$\nu$= 140 eV showing two spin-orbit split components corresponding to Te2-Te3 (gray shading) and Te1 (light blue shading). The least square curve fitting (solid line) has been performed using the Doniach-Sunjic lineshape as in our earlier work [3]. The residual of the fit is shown as a black curve in the top part of the figure.

is shifted to higher $E$ (by 0.63 eV) as expected for lesser negative valency. Moreover, the integrated intensity of the Te2-Te3 peak being almost double of the Te1 peak justifies their identification. Two components in the Te $3d_{5/2}$ core level spectrum have also been reported from x-ray photoelectron spectroscopy [7].

## Supplementary Note 4: Variation of the CDW gap with k$_x$ and k$_y$

The CDW gap observed in the ARPES intensity plot towards the $\Gamma Z$ [6, 8] is shown by a red double arrow in the first slice of Supplementary Fig. S6a (the same is shown in Fig. 4b). A set of $E(k_z)$ ARPES intensity plots parallel to $\Gamma Z$ for different $k_x$ in Supplementary Fig. S6a shows that the occupied band (*13*) shifts towards $E_F$ and consequently the separation $\Delta$ decreases (Supplementary Fig. S6b). This band reaches $E_F$ at $k_x$= 0.4 Å$^{-1}$, indicating the closure of the gap. The EBS at different $k_x$ shown in Supplementary Figs. S6c-g provide the theoretical estimate of $\Delta$ that shows a similar trend as ARPES (Supplementary Fig. S6b). The EBS in Supplementary Fig. S6c shows that the lowest unoccupied band almost reaches $E_F$ and provides an estimate of the CDW gap ($\Delta_{\rm CDW}$) to be 0.35 eV. Based on the former observation, $\Delta_{\rm CDW}$ can be estimated from experiment to be 0.45±0.05 eV. This is in good

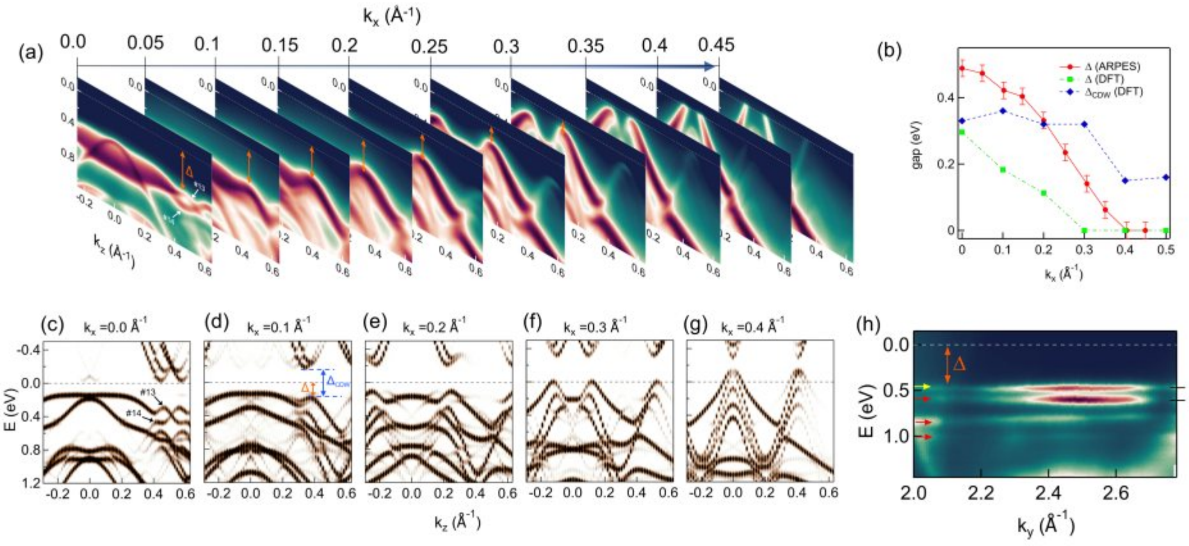


FIG. S6. **Variation of the CDW gap.** (a) The $E(k_z)$ ARPES intensity plots at different $k_x$ values. Δ indicated by the orange double arrow decreases with increasing $k_x$ and the CDW gap closes at $k_x$= 0.4 Å$^{-1}$. (b) Δ from ARPES compared with $\Delta_{\mathrm{CDW}}$ and Δ from DFT. (c-g) EBS [$E(k_z)$] calculated at different $k_x$ portraying the CDW gap variation. (h) $E(k_y)$ plot measured using photon energy dependent scan (h$\nu$= 13-28 eV with 0.1 eV step) at $k_{||}$= 0.48Å$^{-1}$ [cut 1 shown in Fig. 4b of the main text]. The yellow arrow showing the occupied band (*13*) that determines $\Delta_{\mathrm{CDW}}$ and the red arrows indicating higher $E$ bands all remain non-dispersive along $k_y$ showing the quasi-2D character of $LaTe_3$.

agreement with previous ARPES study [6]. While ARPES is unable to measure $\Delta_{\mathrm{CDW}}$ for $k_x$>0 since the unoccupied band moves above $E_F$, the estimate from DFT in Supplementary Fig. S6b shows that it remains almost unchanged up to $k_x$= 0.3 Å$^{-1}$ (Supplementary Fig. S6f). In the non-CDW state, dispersing bands crossing $E_F$ along $\Gamma Z$ show the obvious absence of the CDW gap (Supplementary Fig. S7).

An $E(k_y)$ cut at $k_{||}$= 0.48 Å$^{-1}$(cut 1 shown in Fig. 4b) along the vertical to the $k_x$-$k_z$ plane in Supplementary Fig. S6h shows the occupied band *13* (yellow arrow) that determines the CDW gap does not disperse. Thus the CDW gap remains unchanged along $k_y$. In fact, three other bands at larger $E$ with almost no dependence on the $k_y$ are also observed (red arrows). Absence of dispersion along $k_y$ shows the 2D nature of $LaTe_3$.

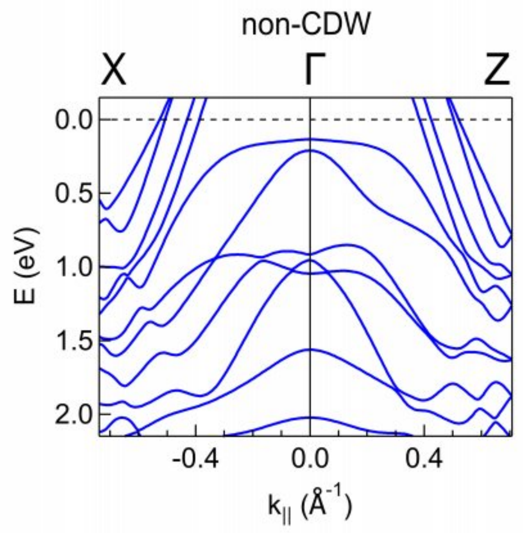


FIG. S7. **Band in the non-CDW state.** Band dispersion along $\Gamma X$ and $\Gamma Z$ directions in the non-CDW state of $LaTe_3$. The primitive unit cell of the non-CDW state with *Cmcm* space group is given by $a= b=$ 13.256Å, $c=$ 4.397Å, $\alpha= \beta=$ 90°, $\gamma=$ 160.99°. Note that $c$ is 7 times less compared to $c'$ in the CDW state shown in Fig. 1a because of the 7 fold modulation.

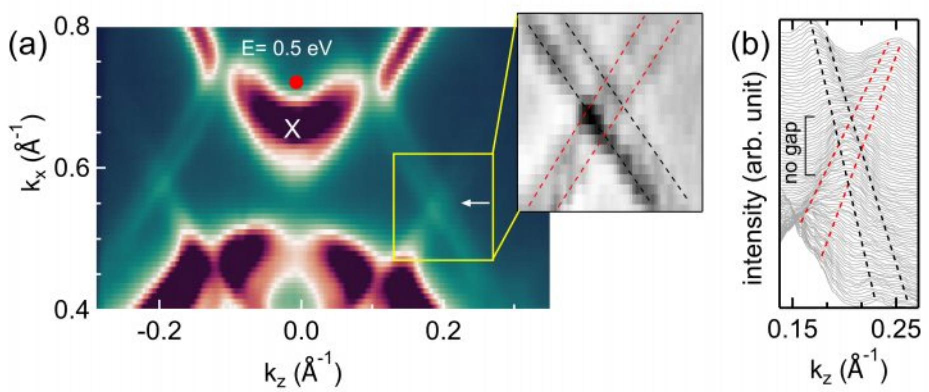


FIG. S8. **Evidence of band crossings.** (a) A constant energy ($E=$ 0.5 eV) isosurface plot measured around the $X$ point. A 2d curvature image of the region marked by a yellow rectangle in the inset highlights the crossing between the two FS branches. (b) A stack of MDCs taken near the crossings in Fig. 2c. The red and black dashed lines in inset of panel **a** and in panel **b** indicate the bilayer split main and shadow bands, respectively.

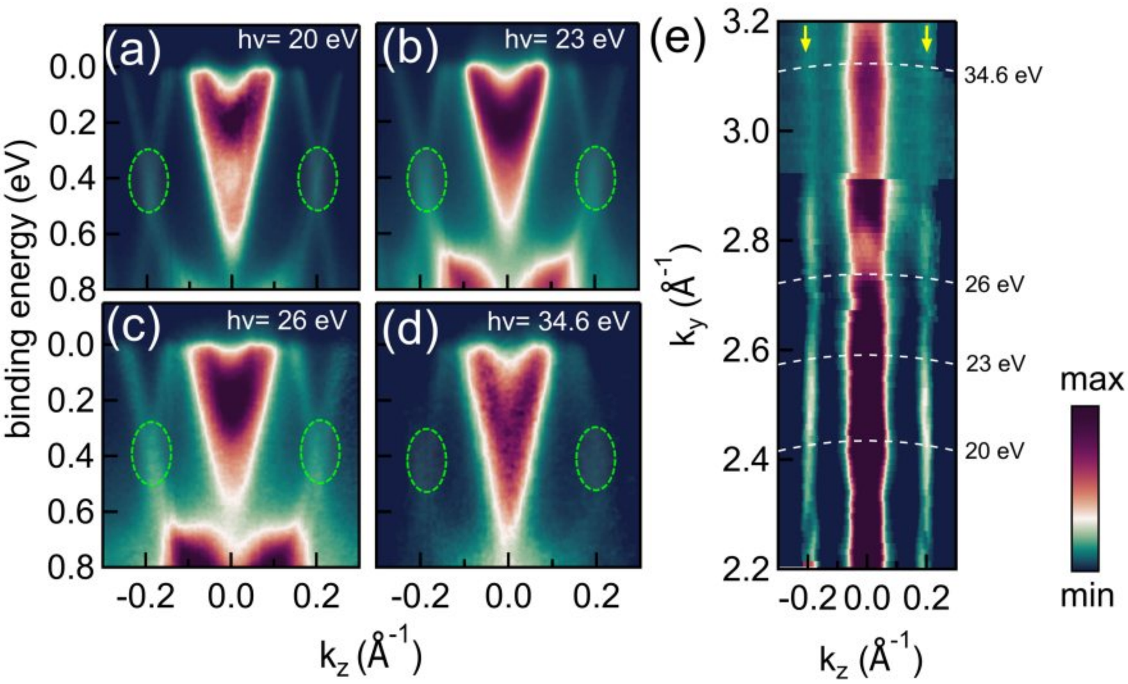


FIG. S9. **Quasi-2D nature of the band crossings.** (a-d) $E(k_z)$ ARPES intensity plots at $k_x$=0.58 Å$^{-1}$ with different photon energies. The band crossings are highlighted by yellow dashed ovals. (e) A constant energy contour at $E$= 0.39 eV. The effective crossings around ±0.2Å$^{-1}$ ($L$ and $R$ merged together) marked by the yellow arrows do not show any dispersion as a function of h$\nu$ indicating their quasi-2D nature.

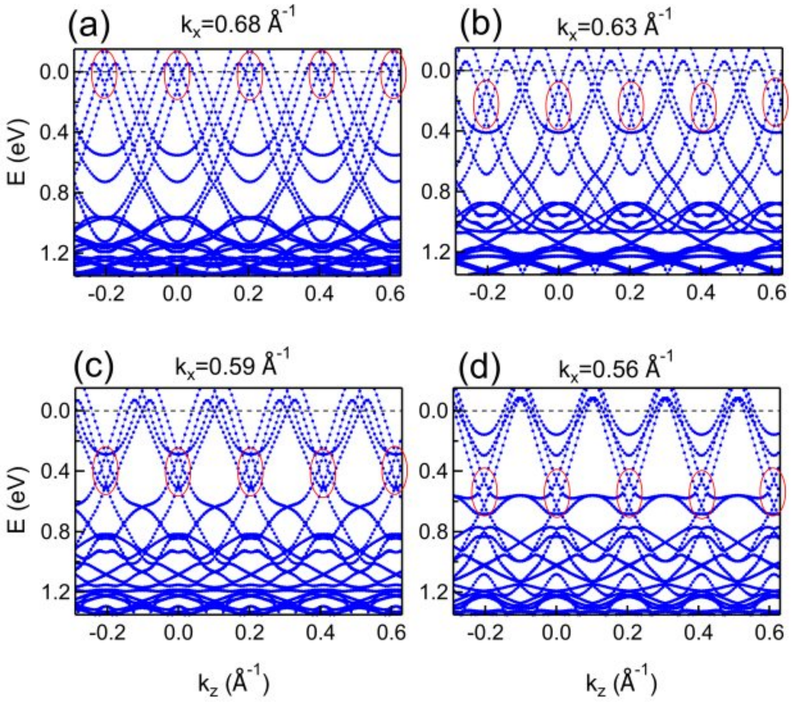


FIG. S10. **Band structure of $LaTe_3$ in the CDW state.** The band structure of $LaTe_3$ in the CDW state for the modulated structure along $k_z$ at $k_x$= (a) 0.68 Å$^{-1}$, (b) 0.63 Å$^{-1}$(c) 0.59 Å$^{-1}$and (c) 0.56 Å$^{-1}$ in an extended zone scheme. The band crossing region in each BZ is highlighted by a red circle.

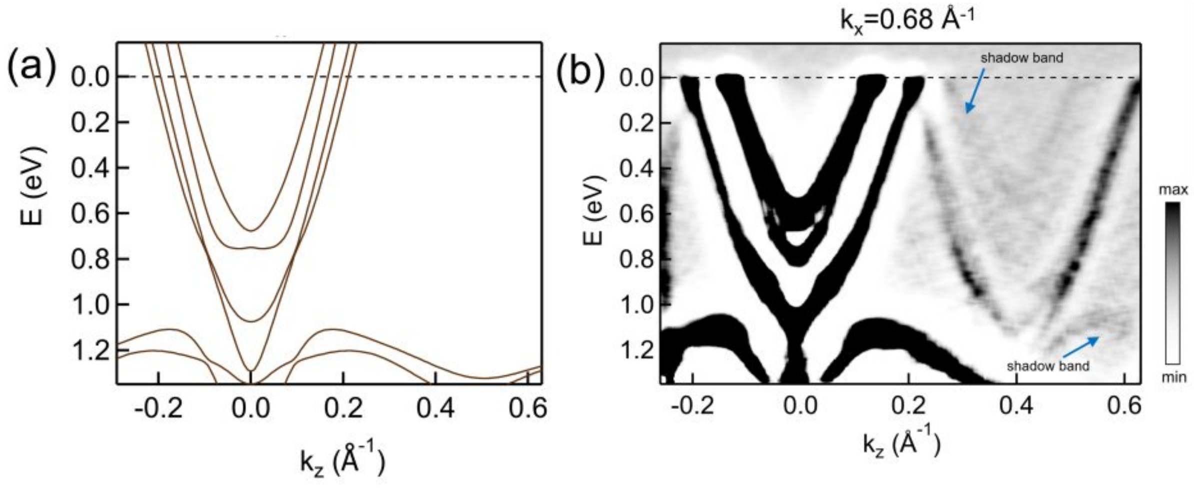


FIG. S11. $E(k_z)$ **bands in the non-CDW and 2d curvature plot from ARPES in the CDW state.** (a) The $E(k_z)$ bands in the non-CDW state of $LaTe_3$. (b) 2d curvature plot of Fig. 2a showing the weak shadow bands of the inner branch (marked by blue arrow).

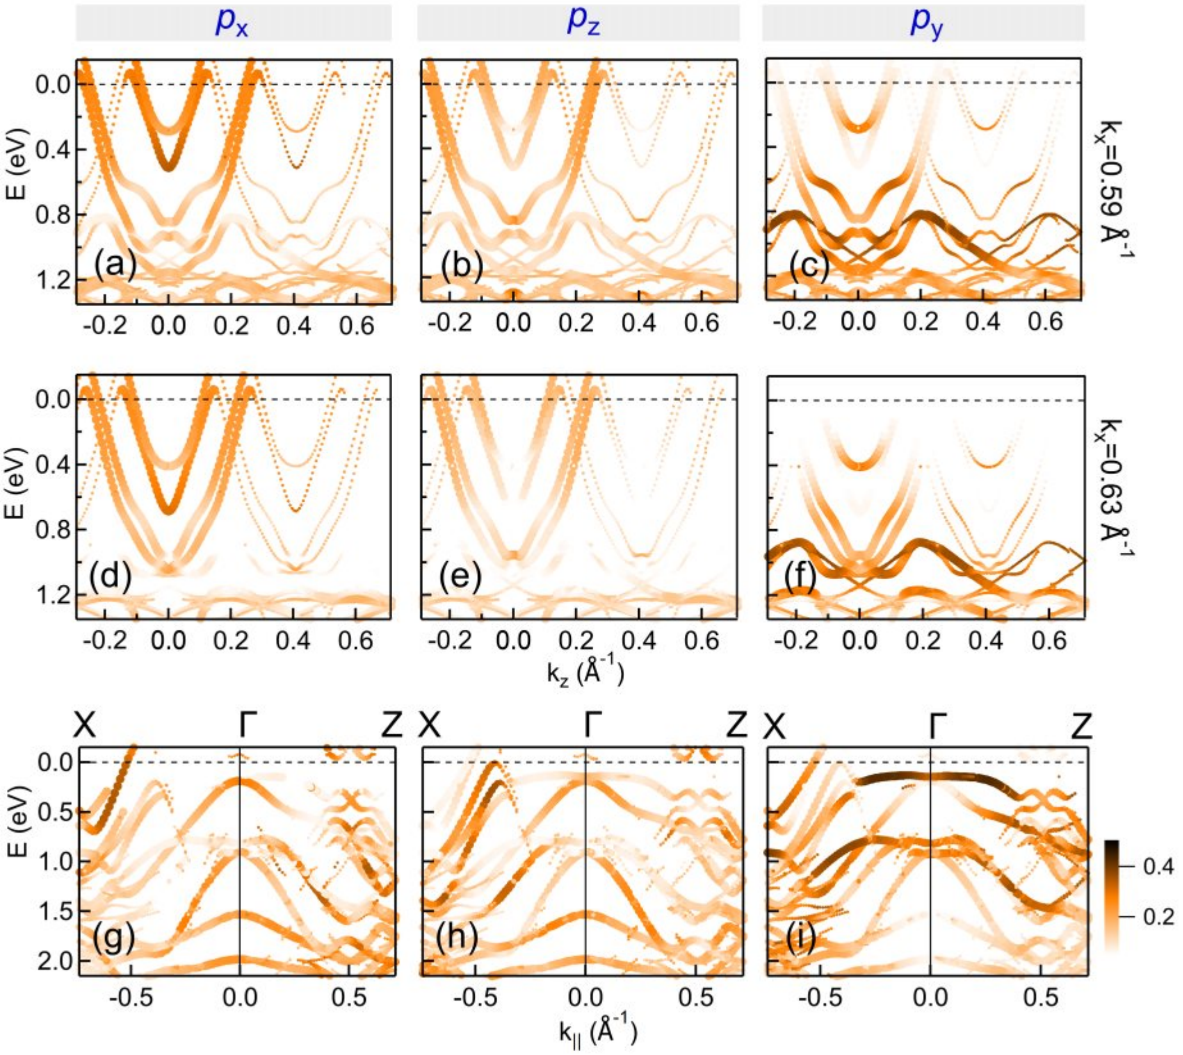


FIG. S12. $p$ **orbital characters of the EBS.** The $p_x$, $p_y$ and $p_z$ orbital characters of the EBS in the CDW state along $k_z$ at (a-c) $k_x$= 0.59 Å$^{-1}$, (d-f) $k_x$= 0.63 Å$^{-1}$and (g-i) along $X\Gamma Z$. The intensity and size of the markers represent the weightage of the orbital characters and the EBS, respectively.

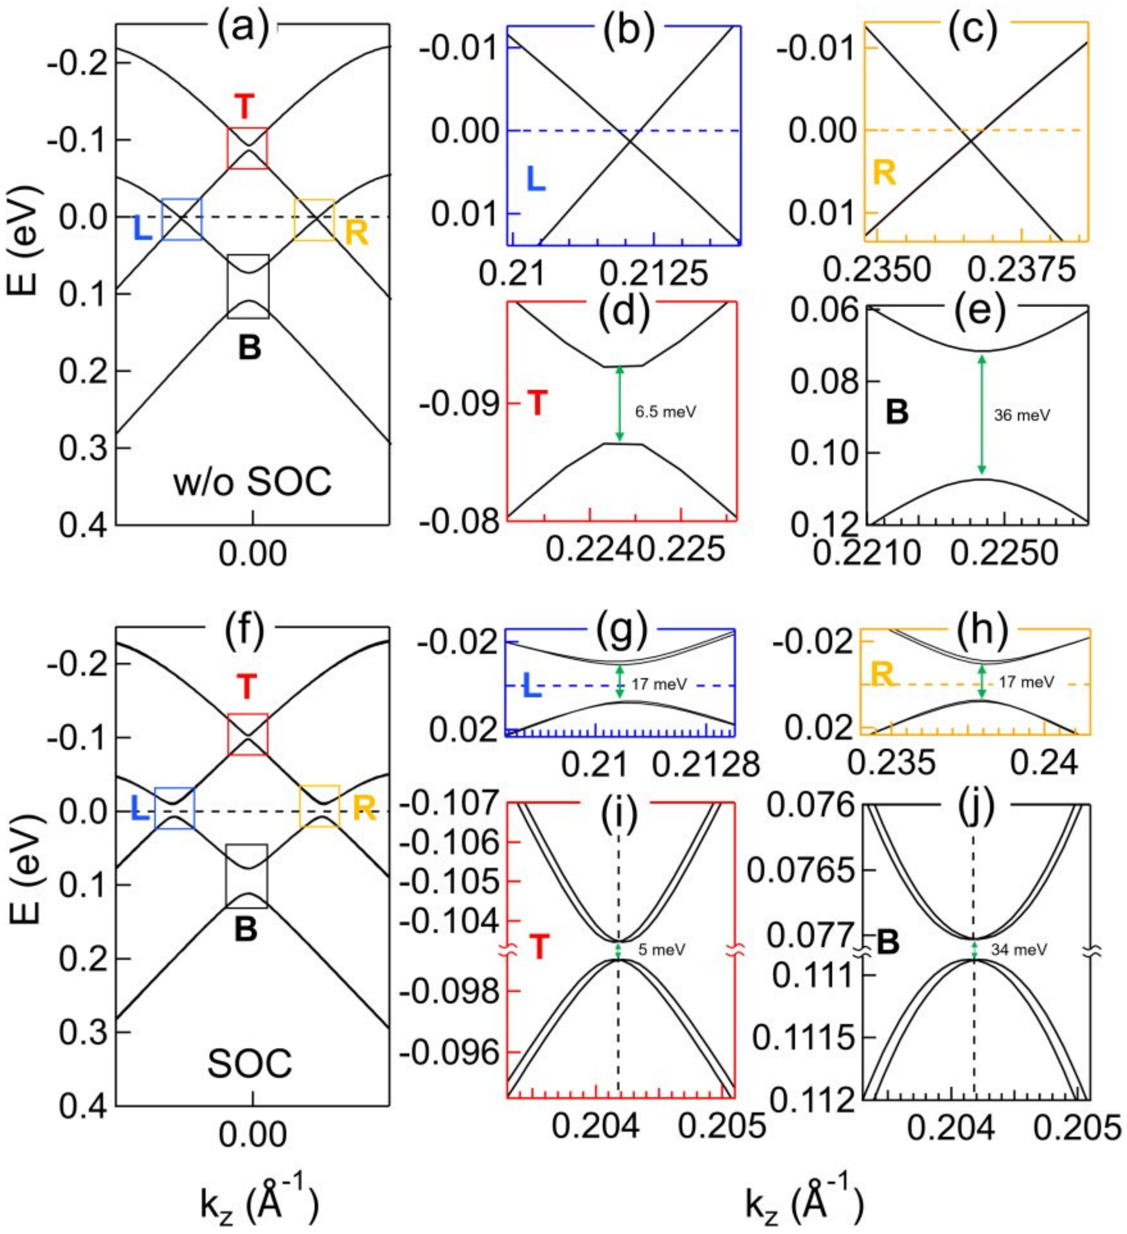


FIG. S13. **Band structure at $k_x$= 0.685 Å$^{-1}$.** (a) $E(k_z)$ bands from DFT at $k_x$= 0.685Å$^{-1}$ without SOC. $E(k_z)$ bands in a small region of the $k$ space within the colored rectangles of panel **a** around (b) $L$, (c) $R$, (d) $T$, and (e) $B$. (f-j) Same as above except that the calculations include SOC. The vertical dashed lines in (i, j) represent the $k_z$ on the $\Gamma_2 X_2$ line.

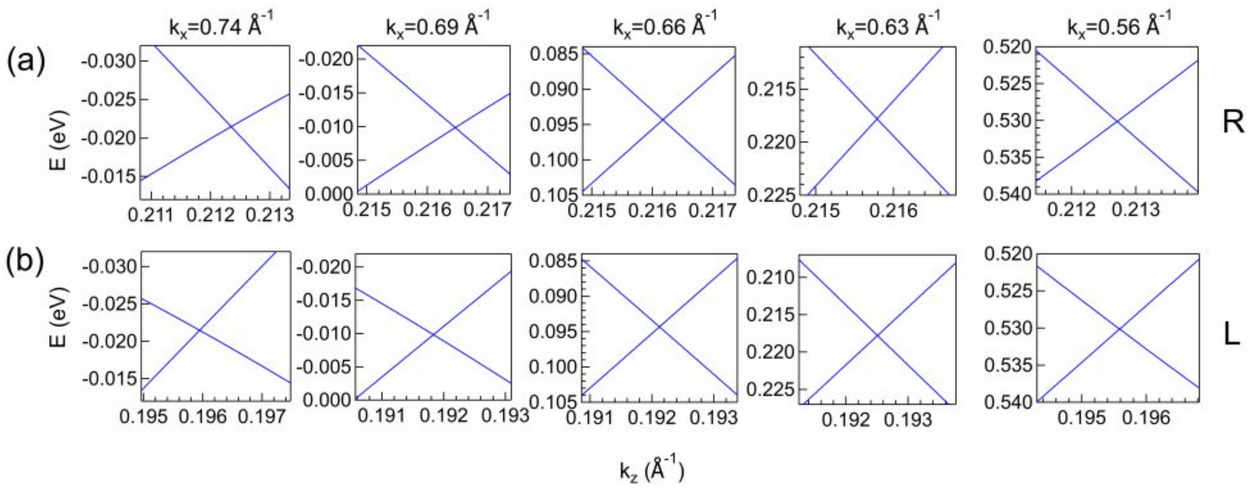


FIG. S14. $L$ **and** $R$ **band crossings at different** $k_x$**.** A series of $E(k_z)$ bands calculated in a small region at different $k_x$ near the (a) $R$ and (b) $L$ crossings without SOC.

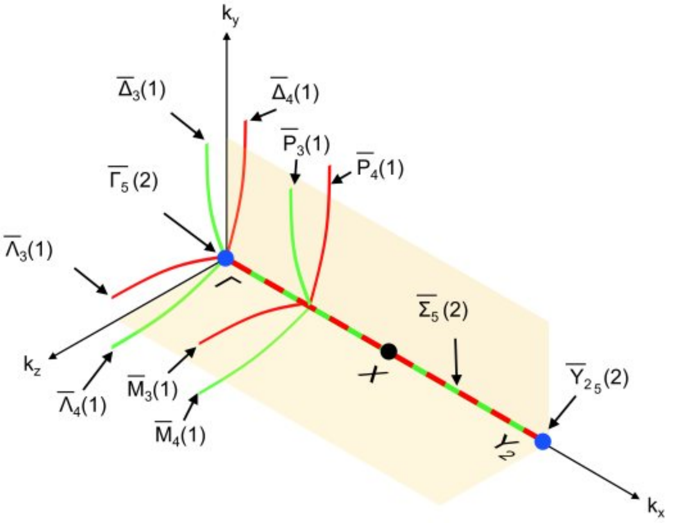


FIG. S15. **Compatibility relations between different** $\boldsymbol{k}$**-paths.** Compatibility relations and band connectivity for $SG$ #40 double space group along different k-paths. The band splittings are shown in the energy axis. The red-green stripped line ($\overline{\Sigma}_5$) shows the Kramers nodal line along the $\Sigma$ line. The TRIM points are denoted by filled blue circles.

TABLE S2. Irreducible representations of $SG$ #40 double space group [10].

| Point/ line of BZ | Irrep (dim) | $\{2_{100}\|000\}$ | $\{m_{010}\|00\frac{1}{2}\}$ | $\{m_{001}\|00\frac{1}{2}\}$ |
|---|---|---|---|---|
| $\Gamma$ (0,0,0) | $\overline{\Gamma}_5(2)$ | $\begin{pmatrix}0 & -1\\ 1 & 0\end{pmatrix}$ | $\begin{pmatrix}0 & -i\\ -i & 0\end{pmatrix}$ | $\begin{pmatrix}-i & 0\\ 0 & i\end{pmatrix}$ |
| $\Sigma$ $(u,u,0)$ | $\overline{\Sigma}_5(2)$ | $\begin{pmatrix}0 & -1\\ 1 & 0\end{pmatrix}$ | $\begin{pmatrix}0 & -i\\ -i & 0\end{pmatrix}$ | $\begin{pmatrix}-i & 0\\ 0 & i\end{pmatrix}$ |
| $Y_2$ (0,0,0) | $\overline{Y_{2}}_5(2)$ | $\begin{pmatrix}0 & -1\\ 1 & 0\end{pmatrix}$ | $\begin{pmatrix}0 & -i\\ -i & 0\end{pmatrix}$ | $\begin{pmatrix}-i & 0\\ 0 & i\end{pmatrix}$ |
| $M$ $(u,u,v)$ | $\overline{M}_3(1)$ | – | $e^{-i\pi(\frac{1}{2}-w)}$ | – |
| | $\overline{M}_4(1)$ | – | $e^{i\pi(\frac{1}{2}+w)}$ | – |
| $\Lambda$ $(0,0,u)$ | $\overline{\Lambda}_3(1)$ | – | $e^{-i\pi(\frac{1}{2}-w)}$ | – |
| | $\overline{\Lambda}_4(1)$ | – | $e^{i\pi(\frac{1}{2}+w)}$ | – |
| $\Delta$ $(-u,u,0)$ | $\overline{\Delta}_3(1)$ | – | – | -$i$ |
| | $\overline{\Delta}_4(1)$ | – | – | $i$ |
| $P$ $(u,v,0)$ | $\overline{P}_3(1)$ | – | – | -$i$ |
| | $\overline{P}_4(1)$ | – | – | $i$ |

TABLE S3. Compatibility relations between irreducible representations of $SG$ #40 double space group along different $k$-paths.

| k-path | Compatibility relations between irreps |
|---|---|
| $\Gamma$:(0,0,0)$\rightarrow\Sigma$:($u$,$u$,0) | $\overline{\Gamma}_5(2)\rightarrow\overline{\Sigma}_5(2)$ |
| $\Sigma$:($u$,0,0)$\rightarrow Y$:(1,0,0) | $\overline{\Sigma}_5(2)\rightarrow\overline{Y}_5(2)$ |
| $\Gamma$:(0,0,0)$\rightarrow\Lambda$:(0,0,$u$) | $\overline{\Gamma}_5(2)\rightarrow\overline{\Lambda}_3(1)\oplus\overline{\Lambda}_4(1)$ |
| $\Gamma$:(0,0,0)$\rightarrow\Delta$:($-u$,$u$,0) | $\overline{\Gamma}_5(2)\rightarrow\overline{\Delta}_3(1)\oplus\overline{\Delta}_4(1)$ |
| $\Sigma$:($u$,0,0)$\rightarrow M$:($u$,$u$,$v$) | $\overline{\Sigma}_5(2)\rightarrow\overline{M}_3(1)\oplus\overline{M}_4(1)$ |
| $\Sigma$:($u$,0,0)$\rightarrow P$:($u$,$v$,0) | $\overline{\Sigma}_5(2)\rightarrow\overline{P}_3(1)\oplus\overline{P}_4(1)$ |

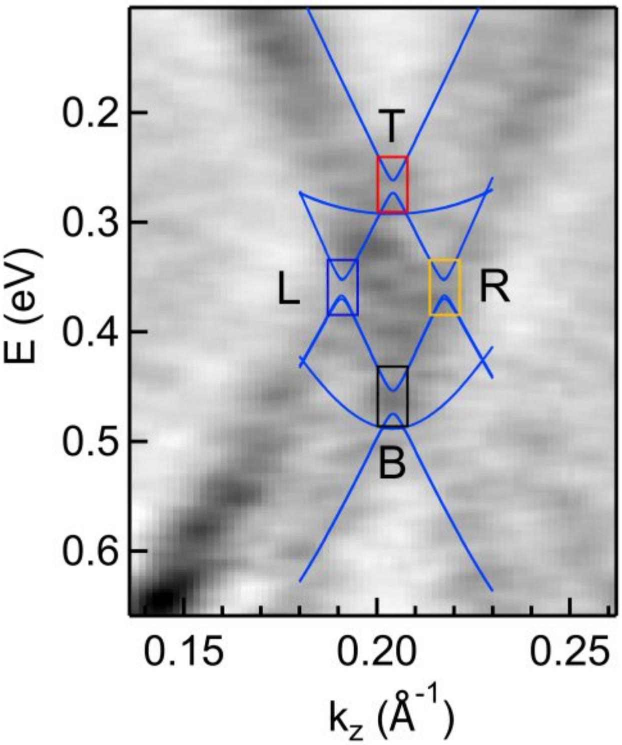


FIG. S16. **Superposition of DFT bands on ARPES.** $E(k_z)$ band dispersion (blue curves) calculated with SOC in Fig. 3i is superimposed on the ARPES intensity plot in Fig. 2f, both at $k_x$= 0.59 Å$^{-1}$. The regions zoomed in Figs. 3l,m are shown within the red and black rectangles, respectively.

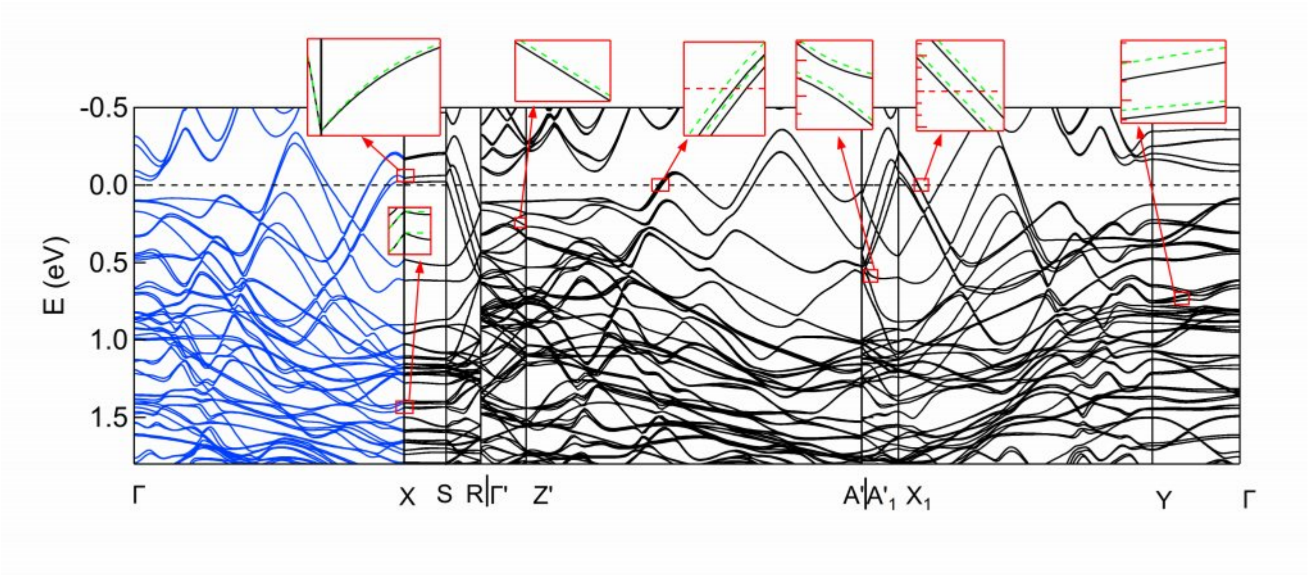


FIG. S17. **Band structure of $LaTe_3$ along the KNL and other high symmetry directions.** Band dispersion calculated with SOC, the high symmetry points of the CDW BZ are indicated at the bottom. The two fold degenerate bands are denoted by blue curves along the KNL ($\Gamma X$). Zoomed regions from the red rectangles that are arbitrarily chosen show the band splittings in all the other directions.

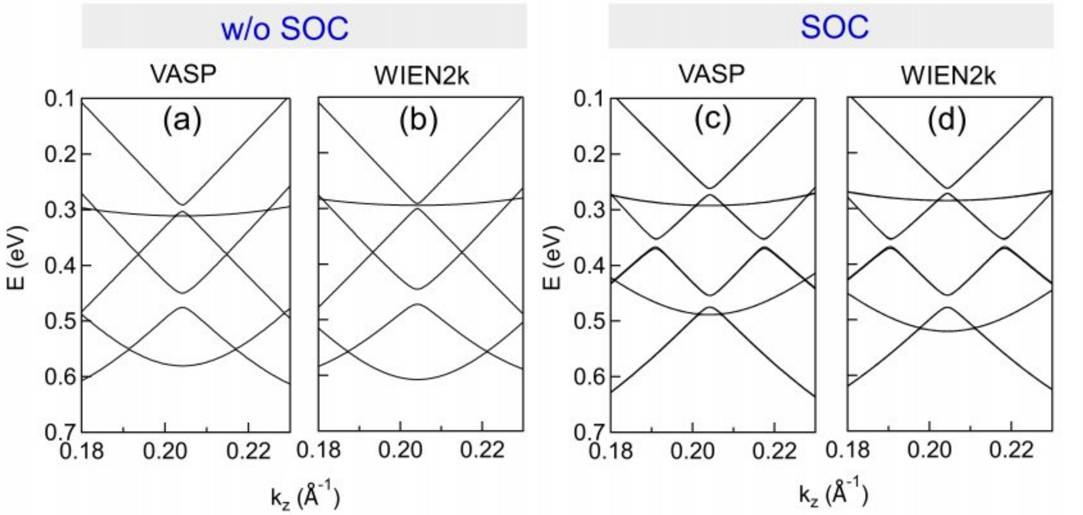


FIG. S18. **Band structures obtained from VASP and WIEN2k.** Comparison of the bands along $k_z$ at $k_x$= 0.59 Å$^{-1}$ in the CDW state calculated using (a,c) VASP and (b,d) WIEN2k.

[1] Komoda, H. et al., High-resolution angle-resolved photoemission study of incommensurate charge-density-wave compound $CeTe_3$, Phys. Rev. B **70**, 195101 (2004).

[2] Malliakas, C. D. and Kanatzidis, M. G., Divergence in the behavior of the charge density wave in $RETe_3$ (RE = rare-earth element) with temperature and RE element, Journal of the American Chemical Society **128**, 12612 (2006).

[3] Sadhukhan, P. et al., Electronic structure of Au-Sn compounds grown on Au(111), Phys. Rev. B **100**, 235404 (2019).

[4] Bader, R. F., Atoms in molecules, Accounts of Chemical Research **18**, 9 (1985).

[5] Bhattacharya, J. and Chakrabarti, A., Electronic and transport properties of heusler alloy based magnetic tunneling junctions: A first principles study, Computational Materials Science **216**, 111852 (2023).

[6] Brouet, V. et al., Angle-resolved photoemission study of the evolution of band structure and charge density wave properties in $RTe_3$ (R=Y, La, Ce, Sm, Gd, Tb, and Dy), Phys. Rev. B **77**, 235104 (2008).

[7] Sarkar, S. et al., X-ray photoelectron spectroscopy study of a layered tri-chalcogenide system LaTe3, *AIP Conference Proceedings*, **2220**, 100005 (2020).

[8] Brouet, V. et al., Fermi surface reconstruction in the cdw state of $CeTe_3$ observed by photoemission, Phys. Rev. Lett. **93**, 126405 (2004).

[9] Setyawan, W. and Curtarolo, S., High-throughput electronic band structure calculations: Challenges and tools, Computational Materials Science **49**, 299 (2010).

[10] Elcoro, L. et al., Double crystallographic groups and their representations on the bilbao crystallographic server, Journal of Applied Crystallography **50**, 1457 (2017).
